# Supplementary material for: Mixed-halide perovskite alloys $\text{CsPb}(\text{I}_{1-x}^{}\text{Br}_x^{})_3^{}$ and $\text{CsPb}(\text{Br}_{1-x}^{}\text{Cl}_x^{})_3^{}$: New insight of configuration entropy effect from first principles and phase diagrams
Source: arXiv:2402.19274 source file (2024-02-29)
Supplement: Supplementary file 1 [file SupportingInformation_c.pdf]

**Supporting Information** for

# Mixed-halide perovskite alloys $CsPb(I_{1-x}Br_x)_3$ and $CsPb(Br_{1-x}Cl_x)_3$ : New insight of configuration entropy effects from first principles and phase diagrams

Fang Pan [1], Junni Zhai [1], Jinyu Chen [1], Lin Yang [1], Hua Dong [2], Fang Yuan [2], Zhuangde Jiang [3], Wei Ren [1], Zuo-Guang Ye [4], Guo-Xu Zhang [5], and Jingrui Li [1,*]

[1] State Key Laboratory for Manufacturing Systems Engineering; Electronic Materials Research Laboratory, Key Laboratory of the Ministry of Education, School of Electronic Science and Engineering, Xi'an Jiaotong University, Xi'an 710049, China

[2] Key Laboratory for Physical Electronics and Devices of the Ministry of Education and Shaanxi Key Lab of Information Photonic Technique, School of Electronic Science and Engineering, Xi'an Jiaotong University, Xi'an 710049, China

[3] State Key Laboratory for Manufacturing Systems Engineering & International Joint Laboratory for Micro/Nano Manufacturing and Measurement Technology, Xi'an Jiaotong University, Xi'an 710049, China

[4] Department of Chemistry and 4D LABS, Simon Fraser University, Burnaby, British Columbia V5A 1S6, Canada

[5] MIIT Key Laboratory of Critical Materials Technology for New Energy Conversion and Storage, School of Chemistry and Chemical Engineering, Harbin Institute of Technology, Harbin 150001, China

[*] jingrui.li@xjtu.edu.cn

## S1 Symmetry analysis of the selected $\sqrt{2}\times\sqrt{2}\times 2$ models

Using $CsPb(X_{10/12}X'_{2/12})_3$ (an 20-atomic model system of which contains 10 X and 2 X′) as an example, we perform the symmetry analysis for the investigated alloys in this section. Figures S1, S2, and S3 show all non-equivalent structures of the $\gamma$ (*Pnma*), $\beta$ (*P*4/*mbm*), and $\alpha$ ($Pm\bar{3}m$) phases, respectively. Figure S4 indicates how the number of non-equivalent structures decreases when the structural symmetry increases.

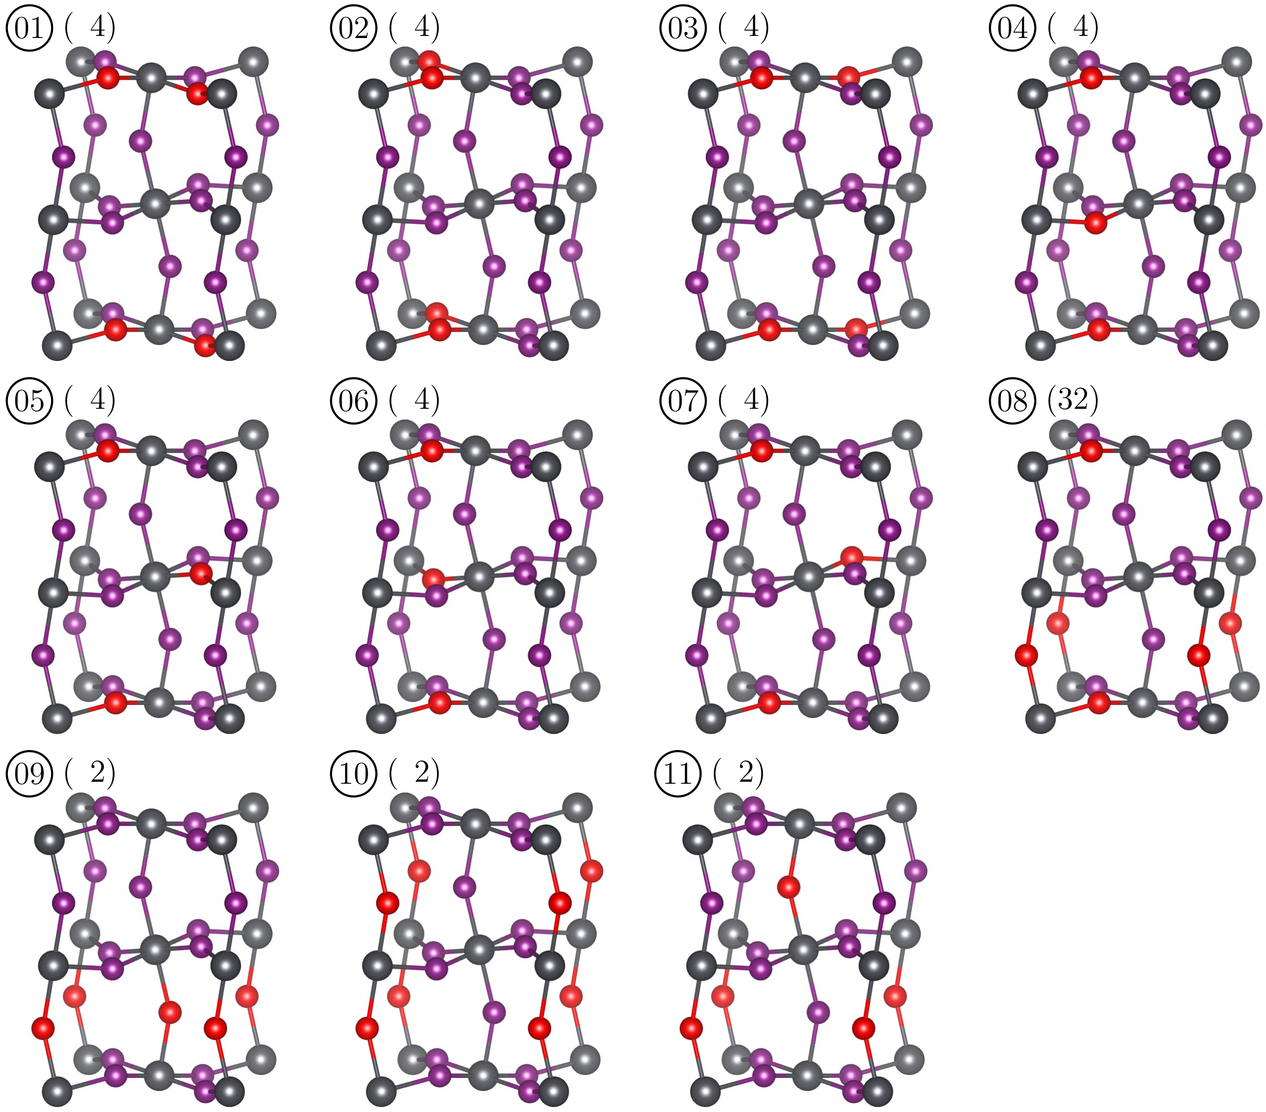


Figure S1: Symmetry-inequivalent structures of $CsPb(X_{10/12}X'_{2/12})_3$ in its $\gamma$ (*Pnma*) phase. The index (in circle) and degree of degeneracy (in parenthese) of each configuration are given. Cs atoms are not shown for clarity, while Pb, X, and X′ are colored in dark gray, purple, and red, respectively.

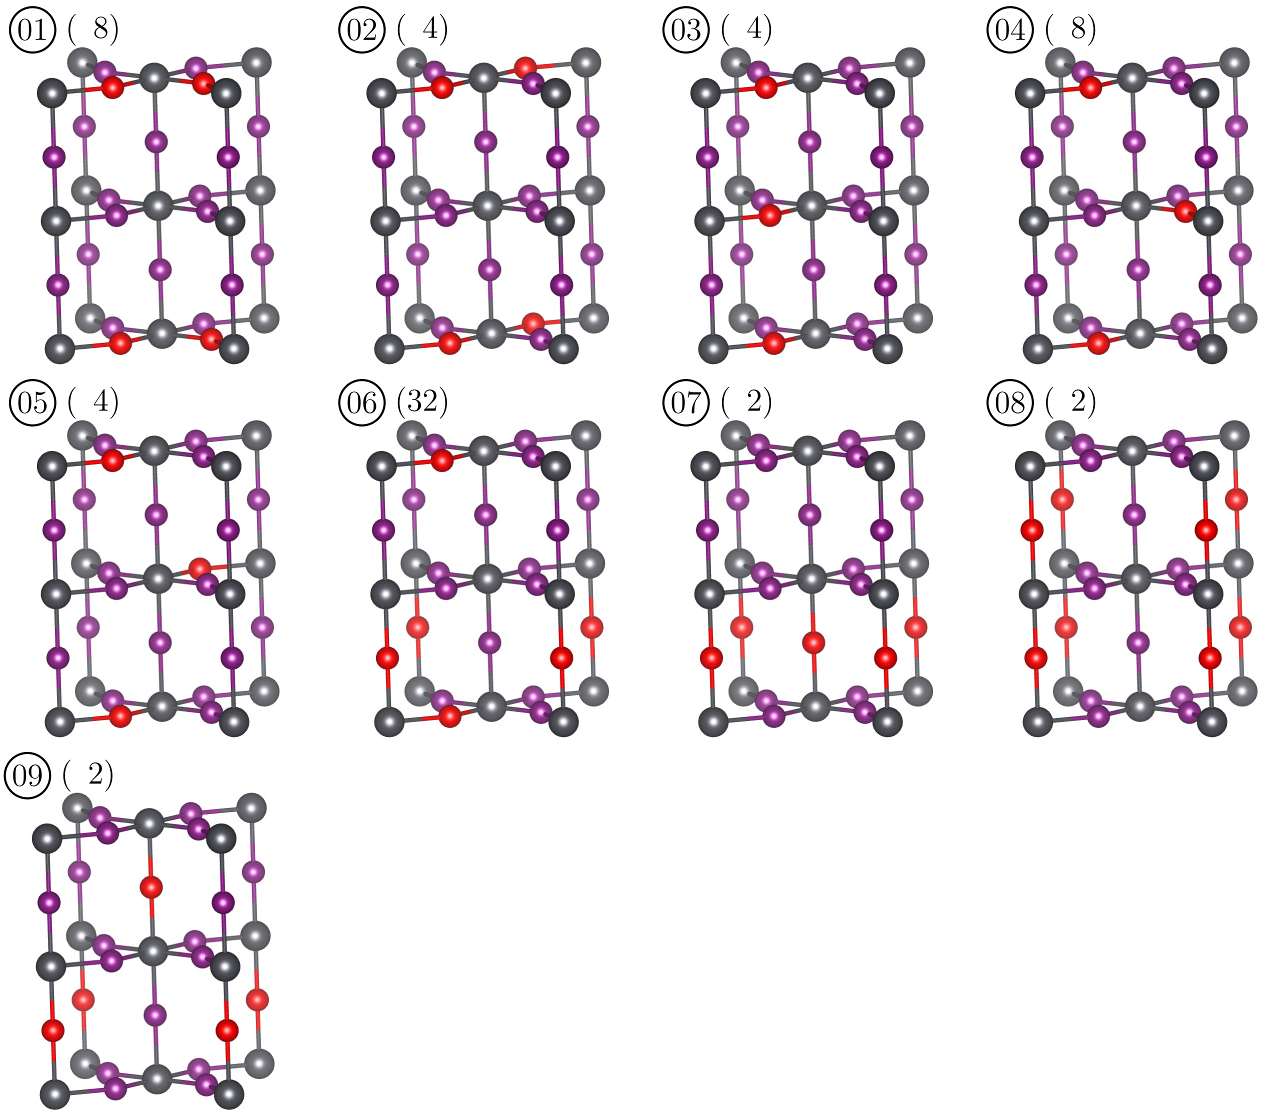


Figure S2: Symmetry-inequivalent structures of $CsPb(X_{10/12}X'_{2/12})_3$ in its $\beta$ ($P4/mbm$) phase. Legends follow Fig. S1.

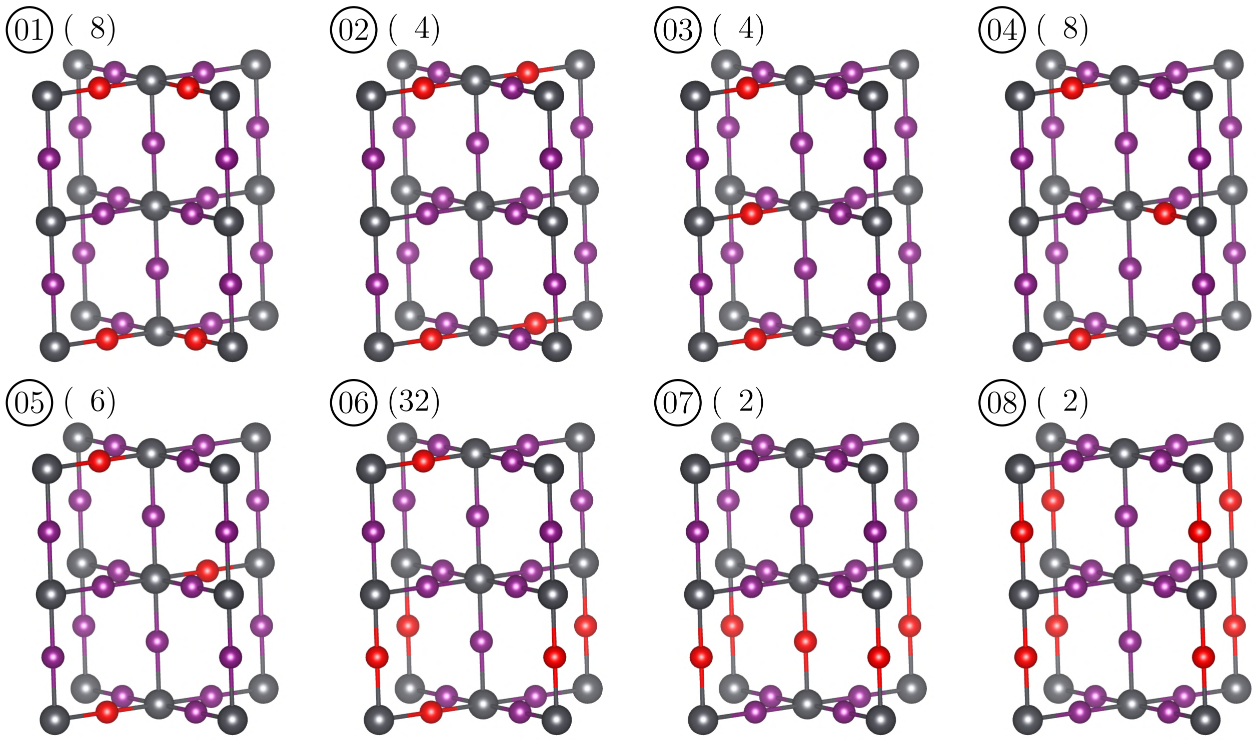


Figure S3: Symmetry-inequivalent structures of $CsPb(X_{10/12}X'_{2/12})_3$ in its $\alpha$ ($Pm\bar{3}m$) phase. Legends follow Fig. S1.

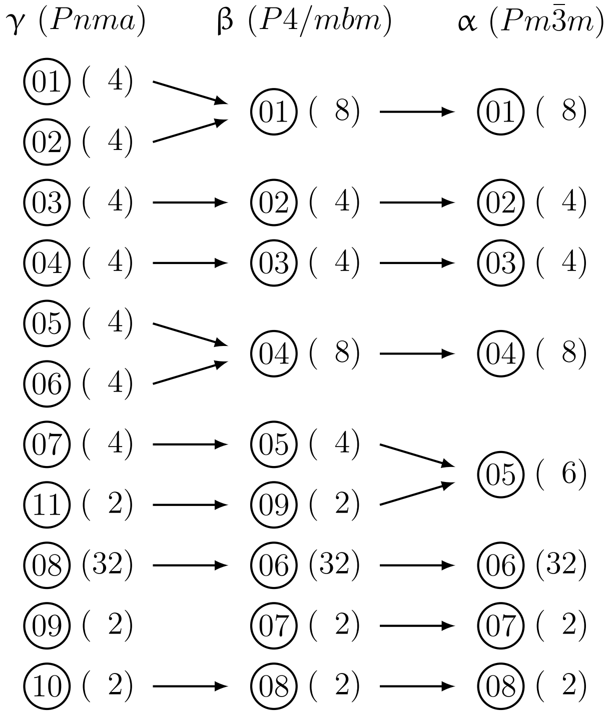


Figure S4: How non-equivalent configurations of lower-symmetry phase merge into equivalent configurations of higher-symmetry phase. Legends follow Fig. S1.

We can see that two pairs (Nos. 1 and 2, and Nos. 5 and 6) of four-fold degenerate structures of $\gamma$ merge into two (No. 1 and No. 4) eight-fold degenerate structures of $\beta$. Similarly, the No. 5 (four-fold degenerate) and No. 9 (two-fold degenerate) of $\beta$ merge into the No. 5 (six-fold degenerate) structure of $\alpha$.

Note: The $\sqrt{2} \times \sqrt{2} \times 2$ model used in this paper is not the best choice for the cubic symmetry, as there is intrinsically difference between the lattice vectors. Therefore we cannot see a significant decrease of non-equivalent configurations when converting from $P4/mbm$ to $Pm\bar{3}m$. Especially, for $x$ or $1-x = \frac{1}{12}, \frac{3}{12}, \frac{5}{12}$, $Pm\bar{3}m$ and $P4/mbm$ exhibit exactly the same symmetry-analysis profile (see Table 1 of the main text). It might seem odd that there are two non-equivalent "cubic" structures with only one minor halide ion as indicated by Table 1. Figure S5 highlights these two non-equivalent sites, and shows how they respectively correspond to two different bi-halide motifs in the unbiased $2 \times 2 \times 2$ model. The degrees of degeneracy of these two bi-halide motifs are 12 (yellow) and 24 (red), respectively. Their ratio exactly equals to $4 : 8$ as in the smaller model. Thus, we can conclude that using the $\sqrt{2} \times \sqrt{2} \times 2$ for the "cubic" phase does not produce incorrectness in symmetry.

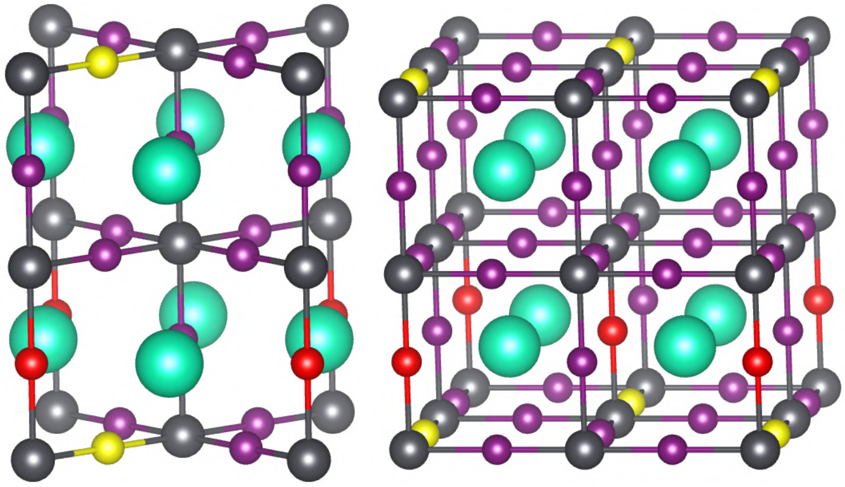

Figure S5: Two non-equivalent X sites (colored in red and yellow) in the $\sqrt{2} \times \sqrt{2} \times 2$ model of the $Pm\bar{3}m$ cubic phase (left) and the corresponding different $X_2$ motifs in the $2 \times 2 \times 2$ model (right). Legends follow Fig. 2 of the main text.

Figure S6 shows that there are three groups of non-equivalent halide ions in the $\delta$ phase of

$CsPbX_3$. The largest number of non-equivalent halides corresponds to the lowest symmetry of this phase and accordingly the largest number of non-equivalent configurations at each composition (see Table 1). Most of the configurations are four-fold degenerate (see Table 1), as each group of equivalent halides contains 4 ions.

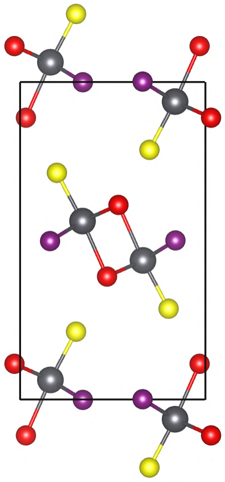

Figure S6: The three different types of halide ions in the δ phase as colored in purple, red, and yellow.

# S2 The lowest- and highest-energy configurations of the perovskite alloys

Figures S7-S12 show the investigated alloy configurations that are associated with the lowest and highest formation energies at each (perovskite) phase and composition. For the cubic ($\alpha$) phase (Figs. S7 and S8), the trend is not obvious due to the narrow energy distribution at each composition [Fig. 3(a) or 4(a)]. Nevertheless, we can see that in the highest-energy structures, halide anions of smaller size [$Br^-$ in $CsPb(I_{1-x}Br_x)_3$ and $Cl^-$ in $CsPb(Br_{1-x}Cl_x)_3$] usually occupy the "in-plane" sites (note: "in-plane" is only a practical concept induced by the $\sqrt{2} \times \sqrt{2} \times 2$ model, meaning the sites at $\{001\}$ planes). In the lowest-energy structures, smaller halides (and therewith also larger halides) occupy both the in-plane and out-of-plane sites, constructing nearest-neighbor iso-halide pairs along the $\langle 110 \rangle$ directions in terms of the cubic lattice which in term lead to iso-halide $\{111\}$ networks. The highest-energy configurations might thus result in lattice distortion, while the lowest-energy configurations largely maintain the structural equivalence along the three primitive cubic lattice vectors. The tetragonal ($\beta$) phase exhibits a distinct character: in the lowest-energy configurations, the smaller halides always prefer to occupy the in-plane sites prior to the out-of-plane ones. The highest-energy configurations exhibit similar character as in the lowest-energy configurations of cubic phase. The orthorhombic ($\gamma$) phase also exhibits an obvious character. It is contradictory to the $\beta$ phase: in the lowest-energy configurations, the larger and smaller halides always prefer to occupy the in-plane and out-of-plane sites, respectively. This is in accordance with the previous results [1]. In the highest-energy configurations, smaller halides only occupy in-plane sites when $x \leqslant \frac{4}{12}$, while for larger $x$ they also occupy out-of-plane sites. Because of the relatively ordered halide alignments, the lowest-energy configurations of both $\beta$ and $\gamma$ phases are usually associated with small degrees of degeneracy. In particular, the structures with the smallest formation energy throughout the whole alloy series, i.e., at $x = \frac{8}{12}$ [Fig. 3(b)] for $\beta$ and $x = \frac{4}{12}$ [Fig. 3(c)] for $\gamma$, exhibit fully ordered, non-degenerate

structure.

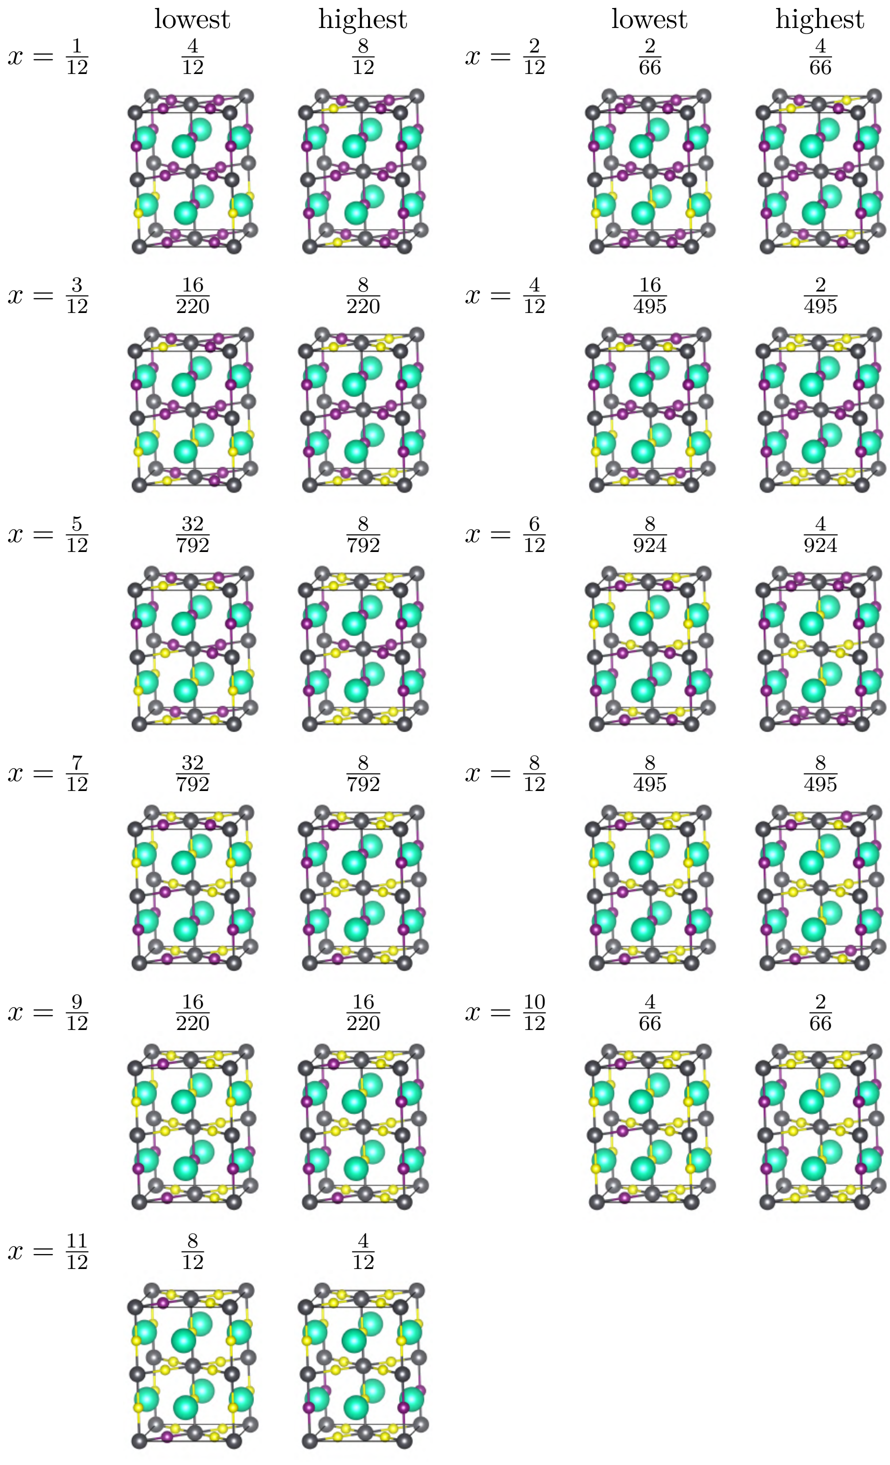


Figure S7: The lowest- and highest-energy structures of $CsPb(I_{1-x}Br_x)_3$ in $\alpha$. Cs, Pb, I, and Br are colored in green, dark gray, purple, and yellow, respectively. The proportion of each configuration in the whole ensemble of the corresponding composition is given.

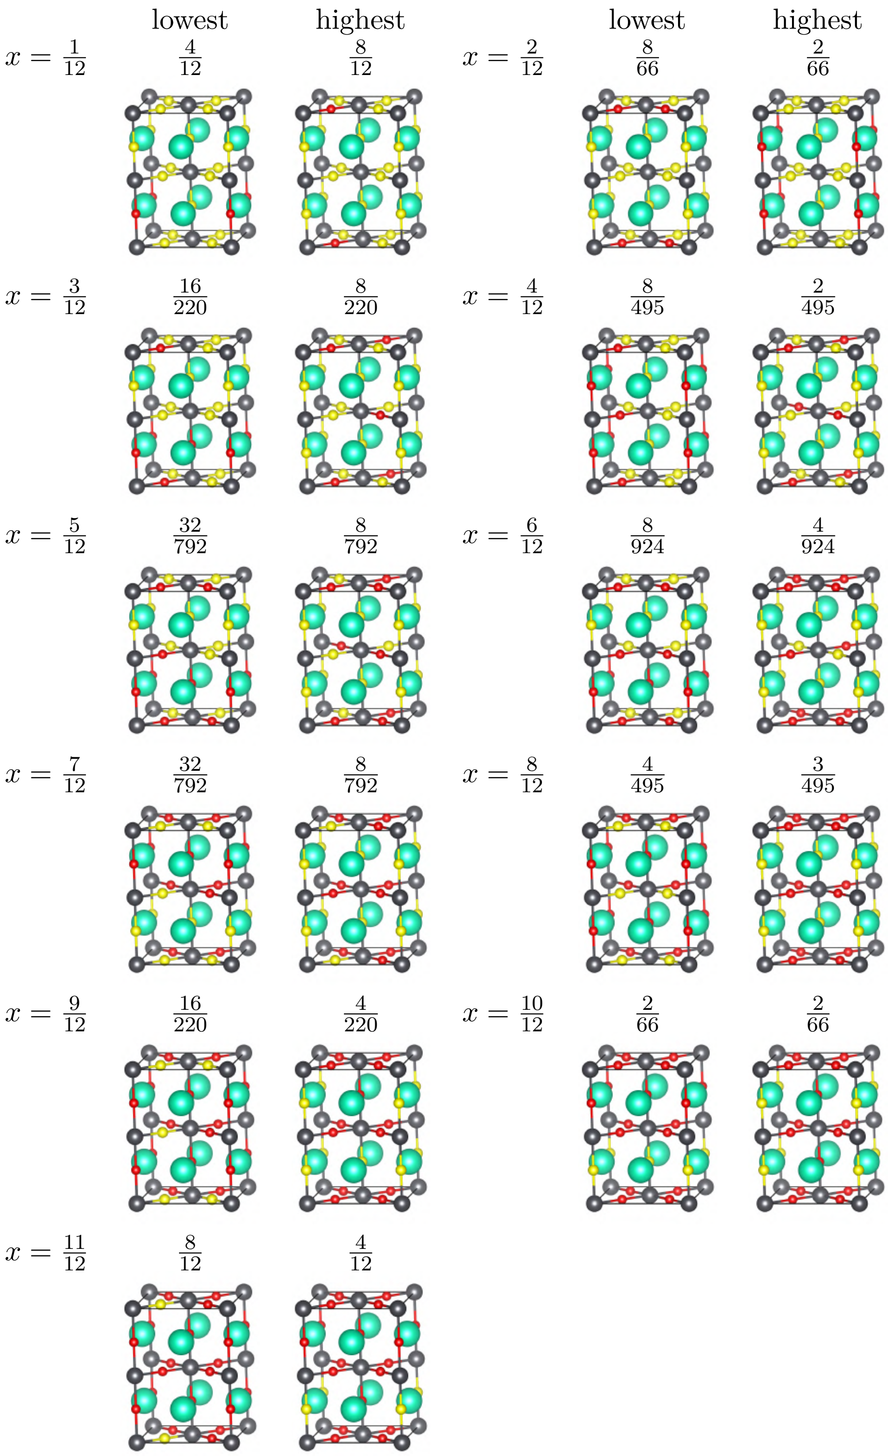


Figure S8: The lowest- and highest-energy structures of $CsPb(I_{1-x}Br_x)_3$ in $\alpha$. Cs, Pb, Br, and Cl are colored in green, dark gray, yellow, and red, respectively. The proportion of each configuration in the whole ensemble of the corresponding composition is given.

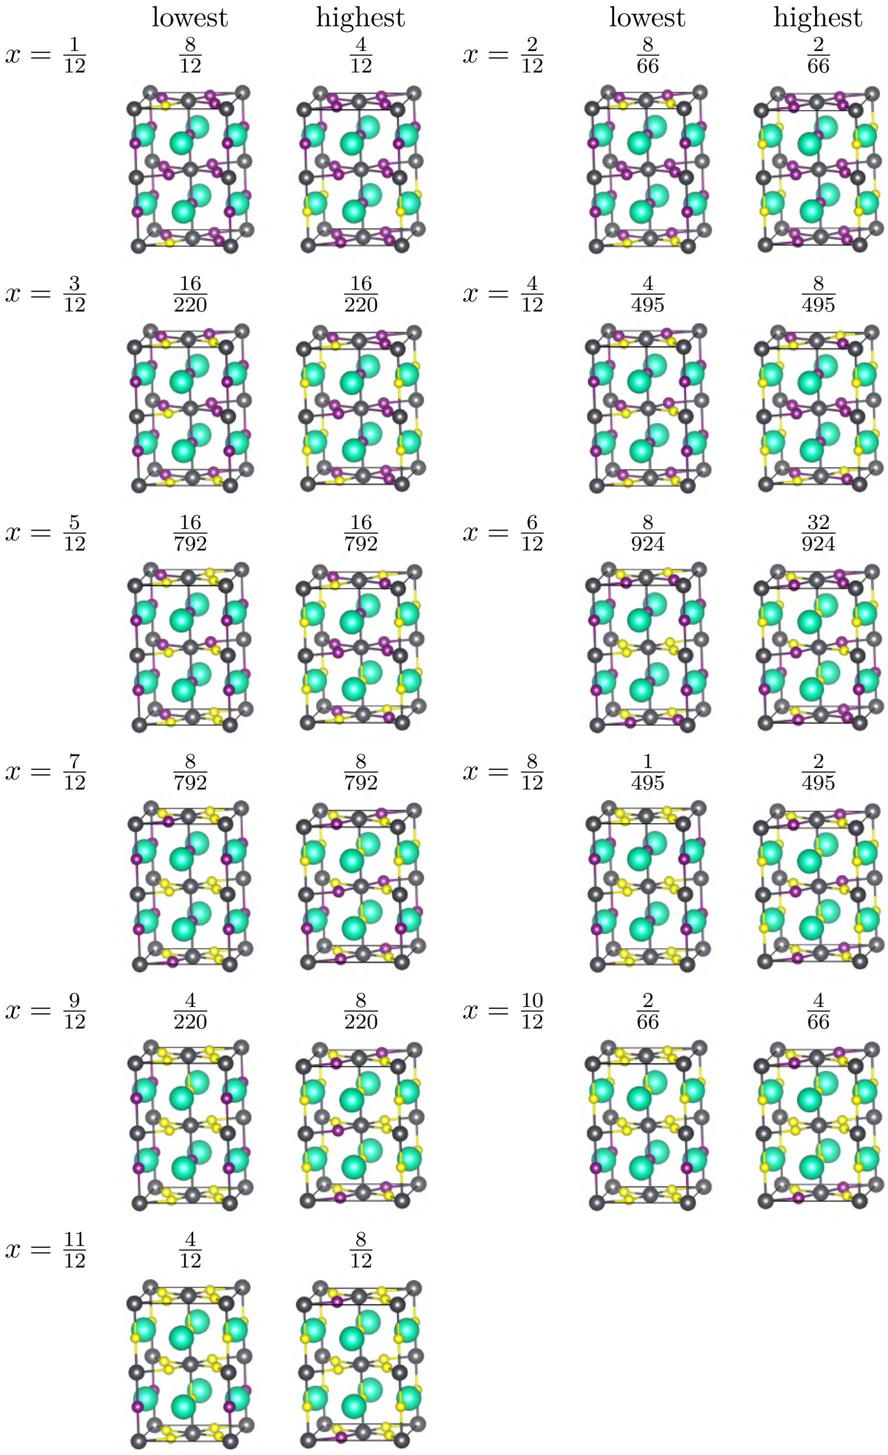


Figure S9: The lowest- and highest-energy structures of $CsPb(I_{1-x}Br_x)_3$ in β. Legends follow Fig. S7.

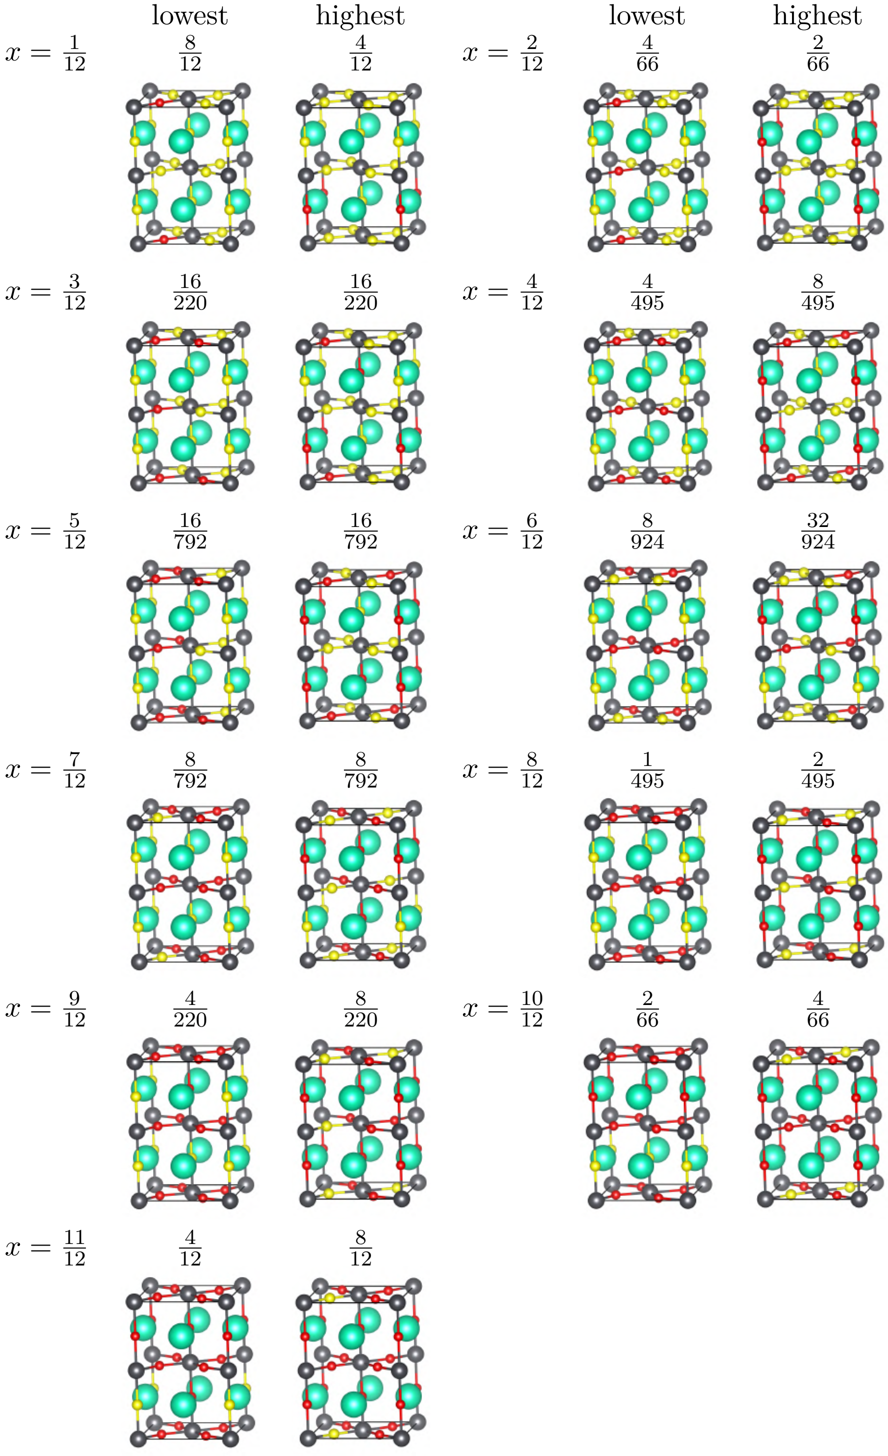


Figure S10: The lowest- and highest-energy structures of $CsPb(I_{1-x}Br_x)_3$ in $\beta$. Legends follow Fig. S8.

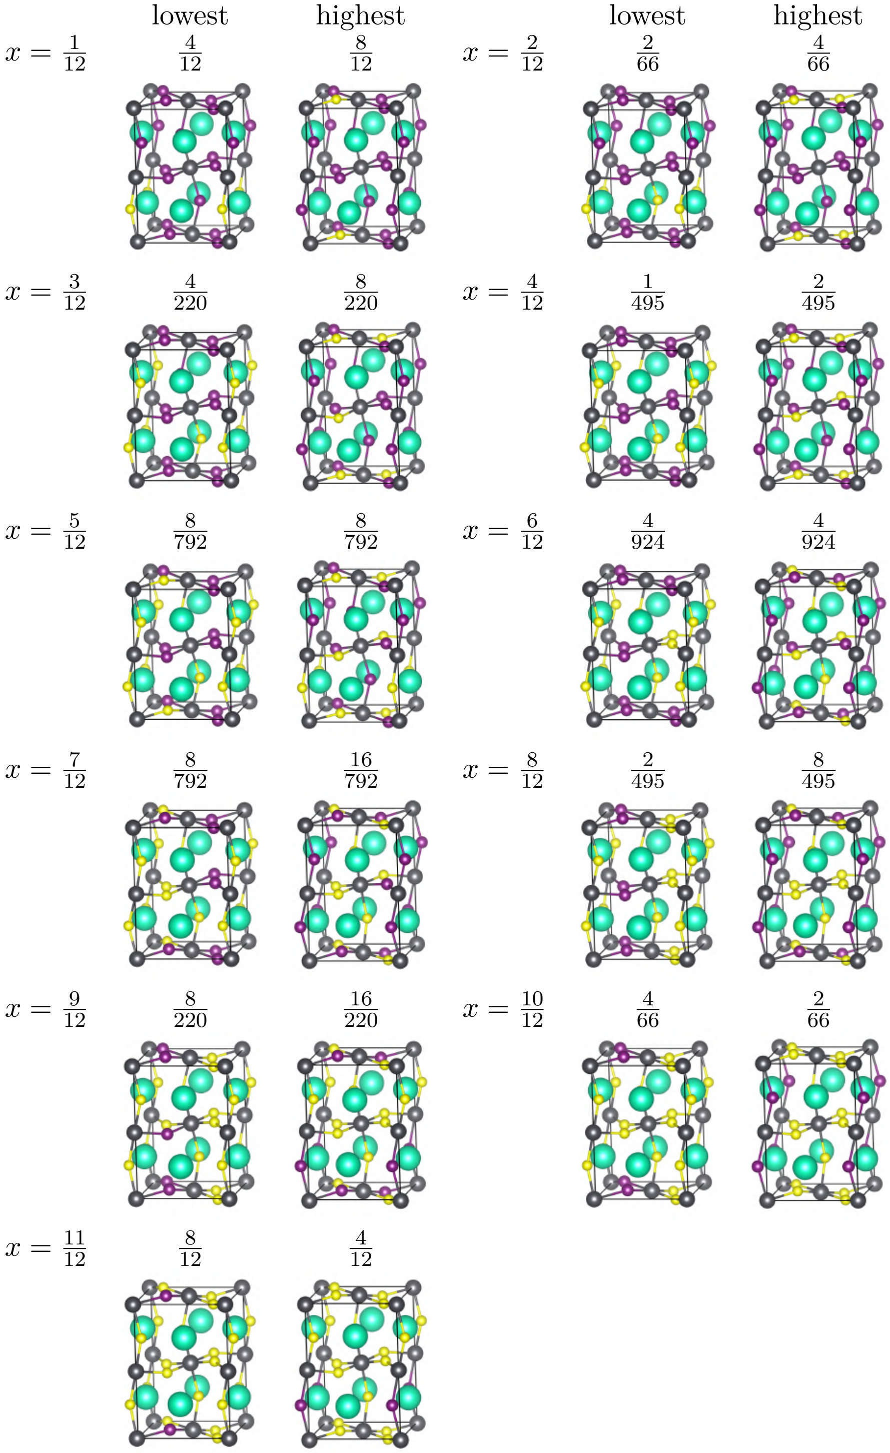


Figure S11: The lowest- and highest-energy structures of $CsPb(I_{1-x}Br_x)_3$ in $\gamma$. Legends follow Fig. S7.

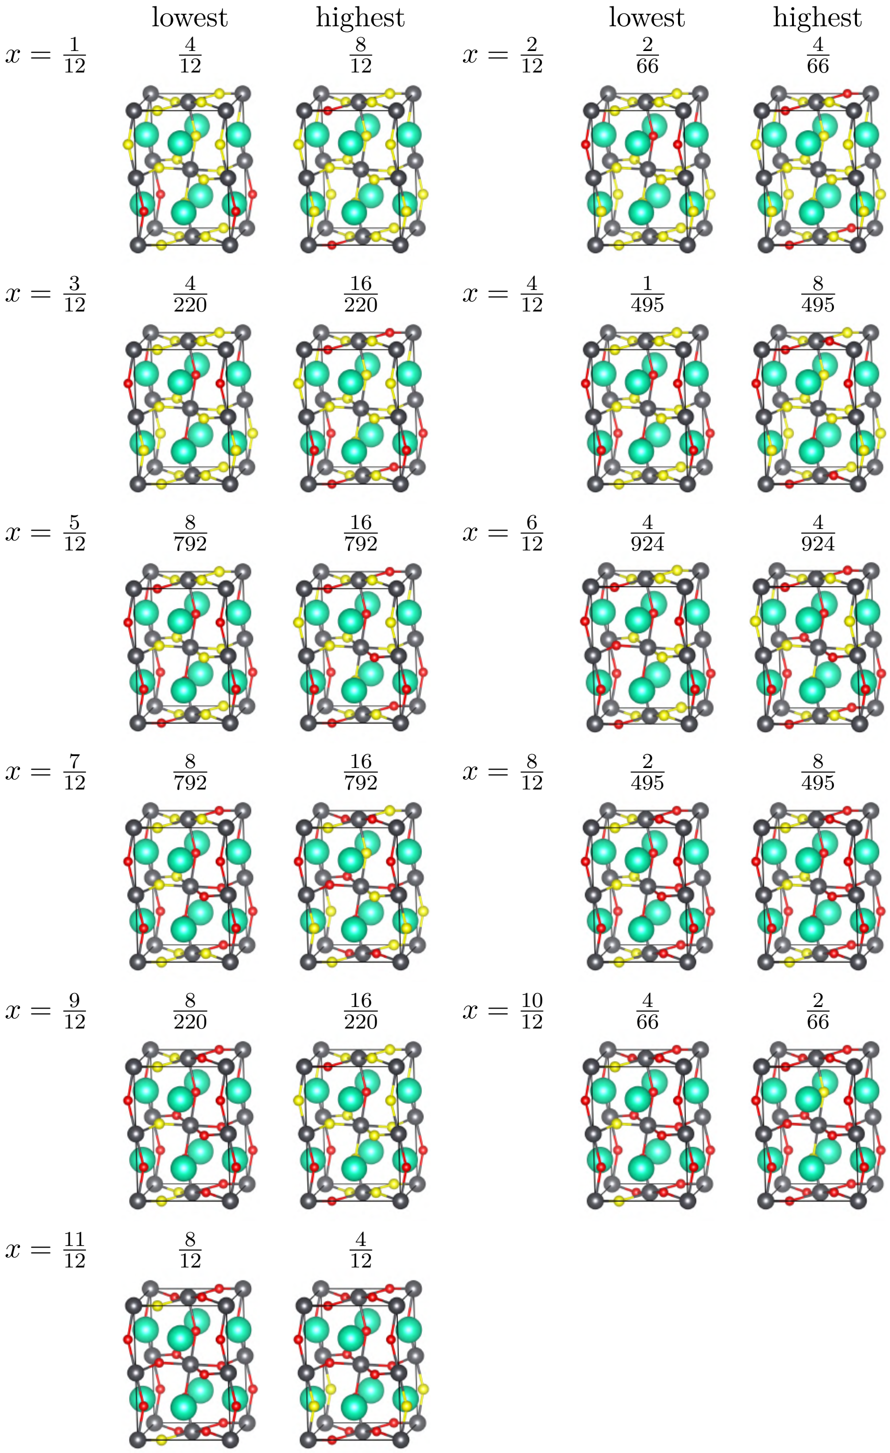


Figure S12: The lowest- and highest-energy structures of $CsPb(I_{1-x}Br_x)_3$ in $\gamma$. Legends follow Fig. S8.

# S3 Finite-size effects

The small 20-atomic model systems might induce finite-size effects. In this section, we briefly study these effects not by increasing the system size, but rather by comparing the 20-atomic results (as in the main text) to the results with smaller model size. To this end, we select the $P4/mbm$ phase, the smallest system of which contain 10 atoms for the pure compounds. Figure S13 shows the formation energy data of both alloys allowed by this smallest model and the energy-level distribution.

(a) $CsPb(I_{1-x}Br_x)_3$

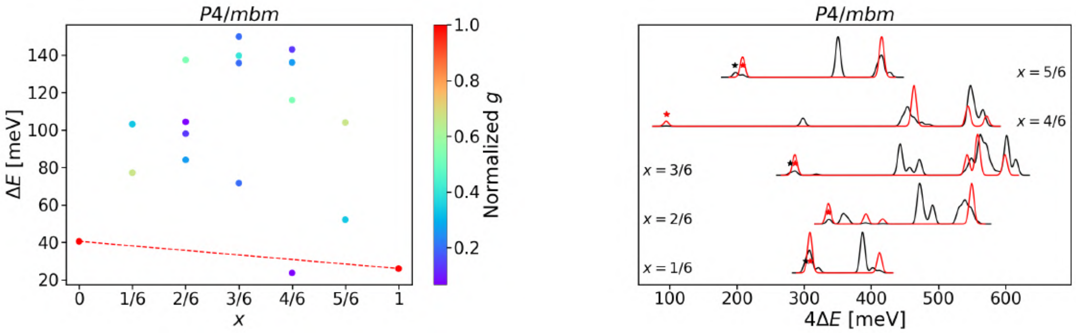


(b) $CsPb(Br_{1-x}Cl_x)_3$

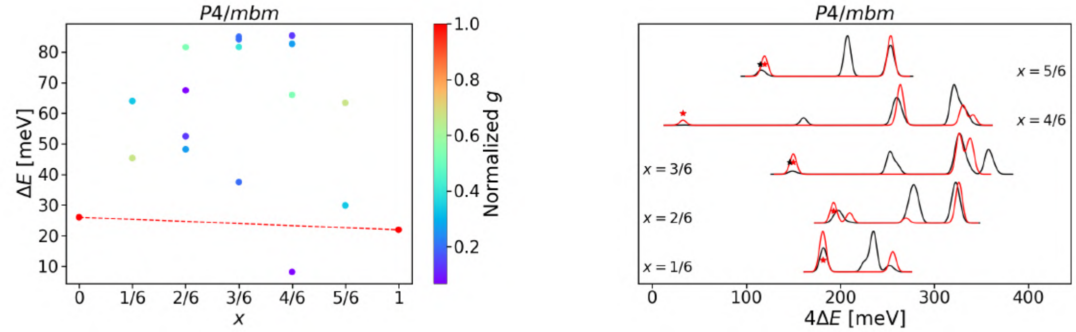


Figure S13: Comparison between the 10- and 20-atomic models for the $P4/mbm$ phase of (a) $CsPb(I_{1-x}Br_x)_3$ and (b) $CsPb(Br_{1-x}Cl_x)_3$. Shown are the formation energies (left, legends follow Fig. 3) and energy-level distribution (right). Both data with the 10- and 20-atomic models are plotted and the lowest energy levels are indicated by stars on the right panel (in red and black, respectively).

As a result of the smaller model system, the left panels of both Fig. S13(a) and (b) exhibit obviously fewer data points than as in Fig. 3(b) left and right, respectively. The major character of formation-energy data are maintained to a certain extend. Obvious difference

between these two models can be seen from the energy-level distribution (right panels of Fig. S13). Because the 10-atomic model system is too small, the minimal formation energies are not exactly the same as with the larger 20-atomic model in some compositions, though the difference is generally small. More importantly, many structures within the mid- and high-energy ranges are missed by the smaller models, because they are disordered and cannot be presented by the smallest models. This will certainly introduce some systematic error when evaluating the thermodynamic properties of the alloy ensembles. Naturally, we can expect that these finite-size effects also exist for our 20-atomic models, which will generally become smaller when the size of model increases.

# S4 Thermodynamic state functions at 400 K

Figure S14 show the thermodynamics state functions at $T = 400$ K. Compared with Fig. 5, the thermodynamic properties of most of the alloys at 400 K are similar to 300 K. The $-TS$ curves and the $F$ convex hulls of both γ and δ phases become deeper, indicating larger entropy stabilization effect than at 300 K. The major difference between Fig. S14 and Fig. 5 can be observed at the β phase of $CsPb(Br_{1-x}Cl_x)_3$. At 300 K, the thermodynamic internal energy $U$ and the minimal formation energy $U_{\mathrm{min}}$ is generally small, while at 400 K the deviation of $U$ from $U_{\mathrm{min}}$ becomes pronounced.

$CsPb(I_{1-x}Br_x)_3$ $CsPb(Br_{1-x}Cl_x)_3$

(a) $Pm\bar{3}m$ phase

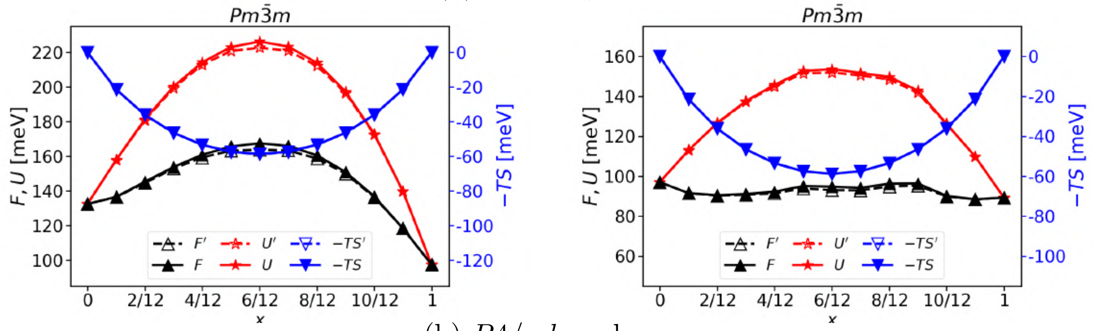


(b) $P4/mbm$ phase

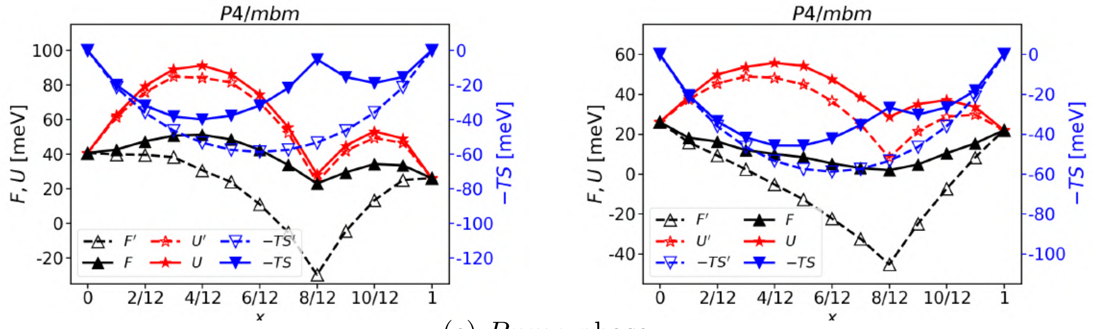


(c) $Pnma$ phase

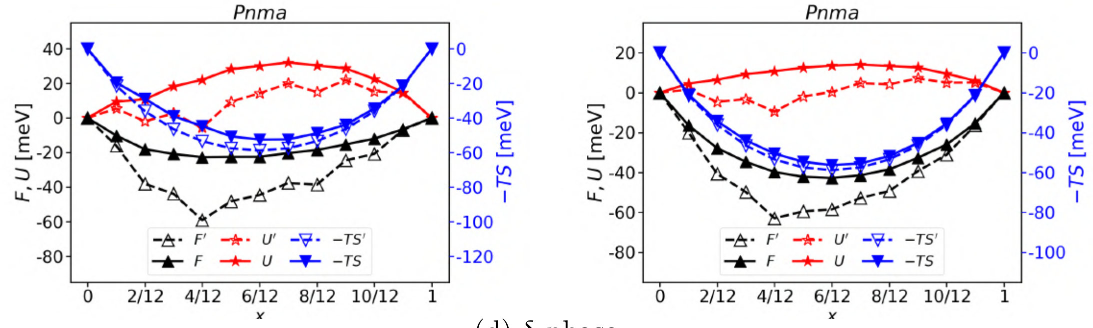


(d) δ phase

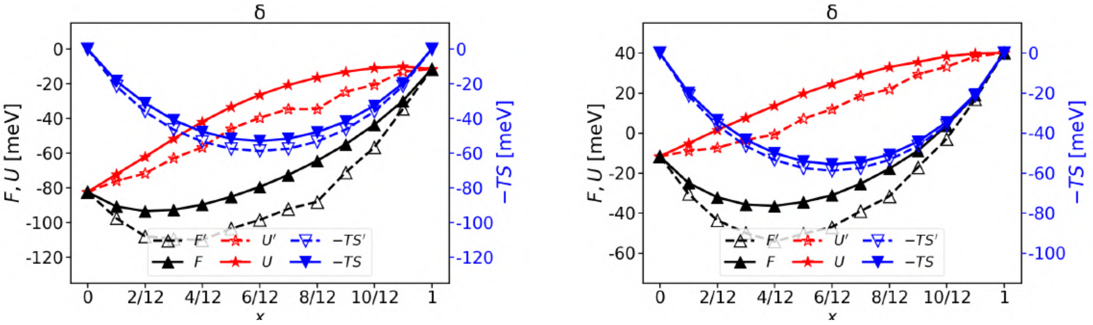


Figure S14: Thermodynamic state functions $F$, $U$, and $S$ of $CsPb(I_{1-x}Br_x)_3$ (left) and $CsPb(Br_{1-x}Cl_x)_3$ (right) in all four phases, (a) α ($Pm\bar{3}m$), (b) β ($P4/mbm$), (c) γ ($Pnma$), and (d) δ ($Pnma$), all compositions, and all configurations at 400 K. Also given are the functions calculated by the traditional approach, $F'$, $U'$, and $-TS'$. Legends follow Fig. 5.

## S5 Band gap distribution

Figures S15-S17 show the band gap distribution of all investigated perovskite alloy phases. For $x = \frac{5}{12}, \frac{6}{12}$ or $\frac{7}{12}$ in the $\alpha$ phase, the band gap of each alloy is distributed within a large range, $\sim 0.25$ eV for $CsPb(I_{1-x}Br_x)_3$ and $\sim 0.10$ eV for $CsPb(Br_{1-x}Cl_x)_3$ , while the formation energy distribution is narrow as alluded to in the main text. Differently, we can generally observe larger energy distribution in other series, and the band gap distribution in the low-energy region is narrow.

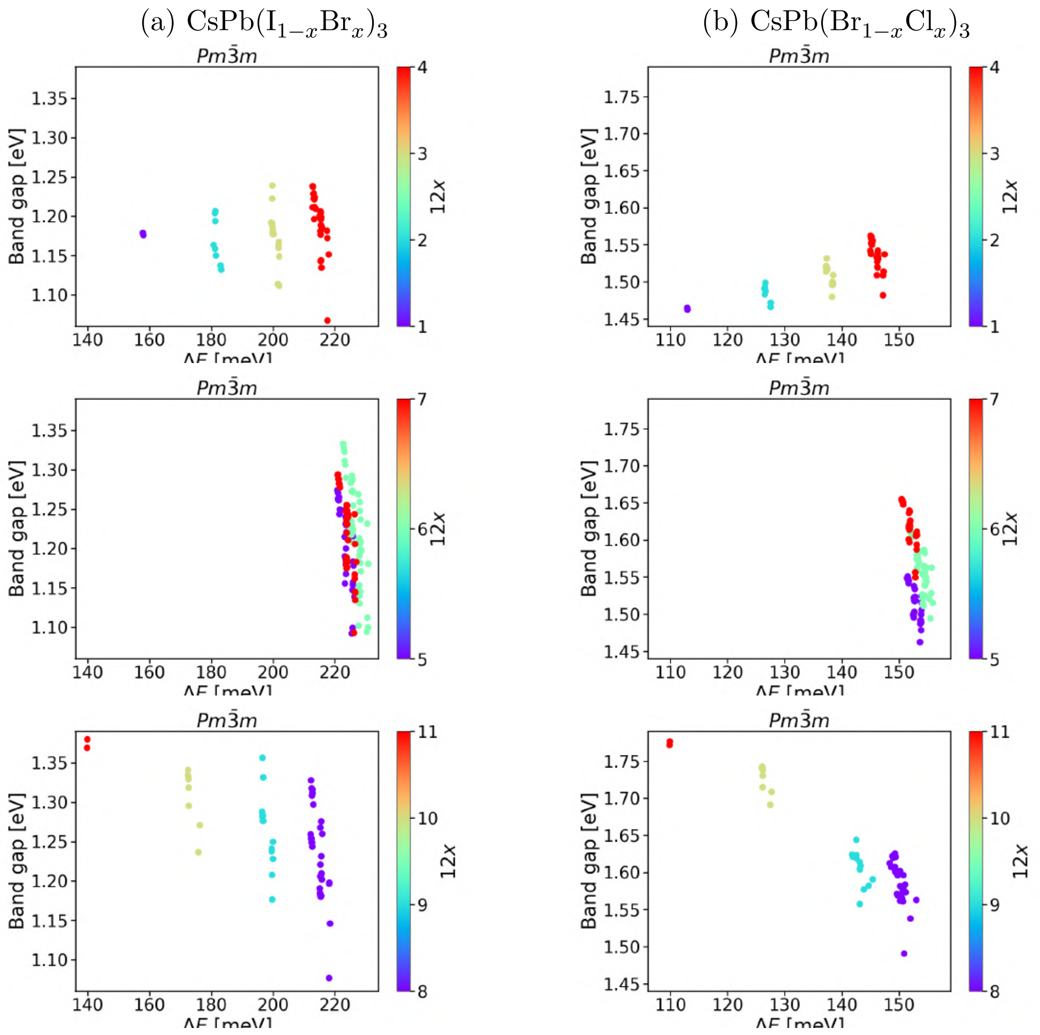


Figure S15: Band gap and formation energy distribution of (a) $CsPb(I_{1-x}Br_x)_3$ and (b) $CsPb(Br_{1-x}Cl_x)_3$ in $\alpha$ phase. Different compositions $x$ are colored differently — from top to bottom: $x \in \left[\frac{1}{12}, \frac{4}{12}\right]$, $x \in \left[\frac{5}{12}, \frac{7}{12}\right]$, and $x \in \left[\frac{8}{12}, \frac{11}{12}\right]$.

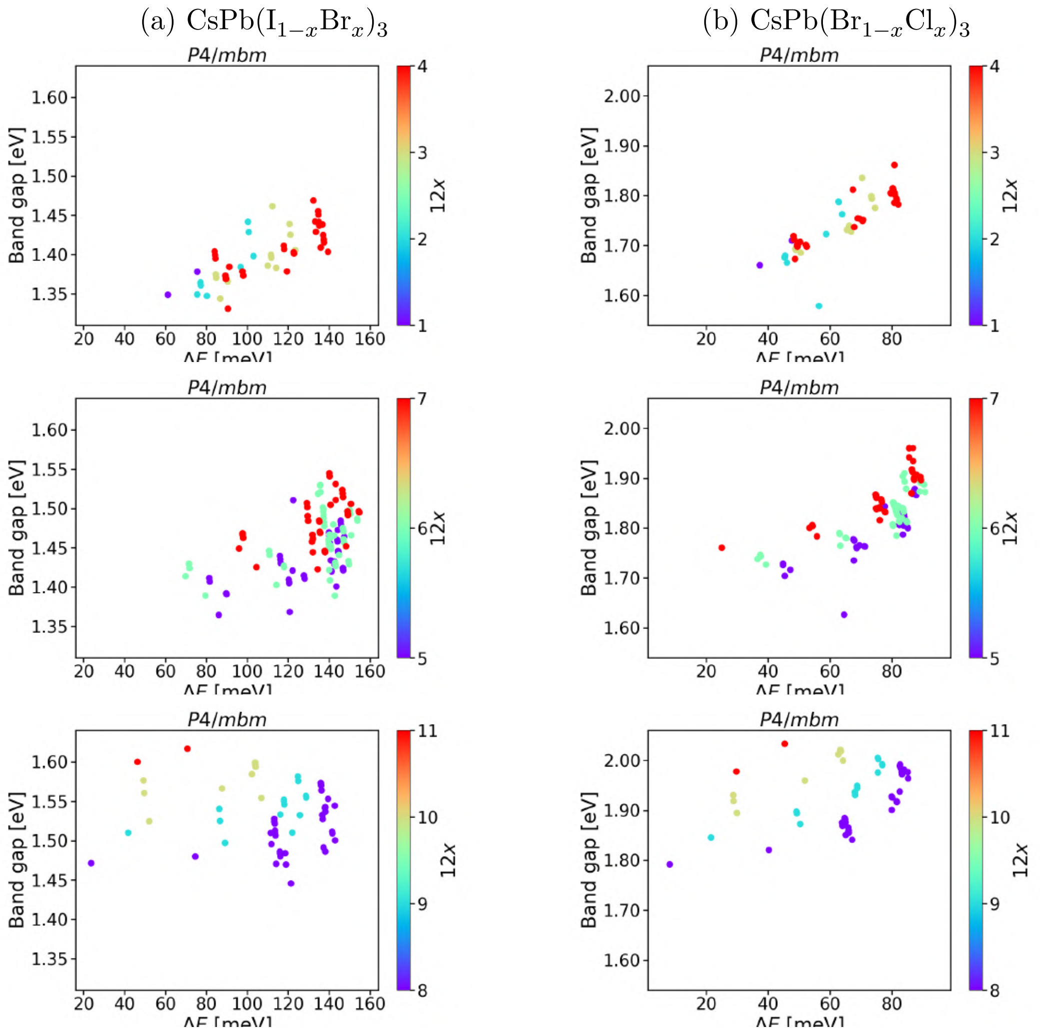


Figure S16: Band gap and formation energy distribution of (a) $CsPb(I_{1-x}Br_x)_3$ and (b) $CsPb(Br_{1-x}Cl_x)_3$ in β phase. Legends follow Fig. S15.

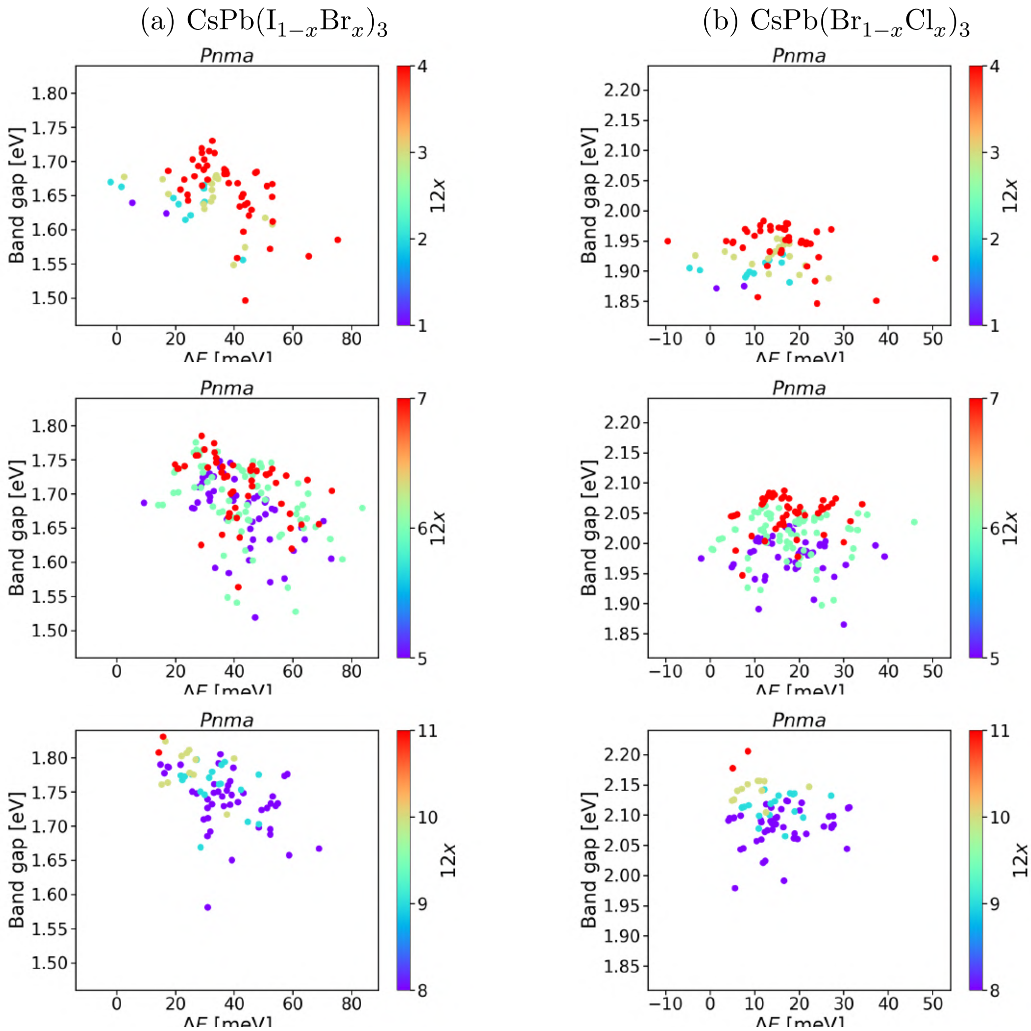


Figure S17: Band gap and formation energy distribution of (a) $CsPb(I_{1-x}Br_x)_3$ and (b) $CsPb(Br_{1-x}Cl_x)_3$ in $\gamma$ phase. Legends follow Fig. S15.

# References

(1) Laakso, J.; Todorović, M.; Li, J.; Zhang, G.-X.; Rinke, P. Compositional engineering of perovskites with machine learning. *Phys. Rev. Materials* **2022**, *6*, 113801.
